# Supplementary material for: Minimizing the Influence of Misinformation via Vertex Blocking
Source: arXiv:2302.13529 source file (2023-02-27)
Supplement: Supplementary file 1 [file appendix.tex]

\clearpage

\appendix 

\section{Appendix}

\subsection{Proofs of Theorems}

\vspace{1mm}
\noindent \textbf{Proof of Theorem~\ref{theo:localup}.}
If $u$ is blocked, for any vertex $x\in N^{out}_u$, $\mathcal{P}^G(x,S)$ will not change if $x$ is a seed, and $\mathcal{P}^G(x,S)$ will decrease otherwise. %, because of the decreasing of $\mathcal{P}^G(u,S)$. 
Thus, the decreasing of $\mathcal{P}^G(x,S)$ will decrease the activation probability of all the out-neighbors of $x$.
Iteratively, the probabilities of all the vertices that $u$ can reach will decrease.
\hfill  $\square$

\subsection{Additional Results}
We report the following results for better reproducibility.
%Due to the space limit, we report the additional experiments under the widely used TR model.
%The trends under WC model are similar to that under TR model.

\noindent \textbf{Varying Error Parameter $\epsilon$ for IP.}
%Note that we cannot set $\epsilon$ by 0 due to float-point error in implementation, while it can be set by a small value, e.g., $\epsilon = 10^{-9}$.
%As real numbers cannot be accurately represented in a fixed space in general, 
Due to floating-point error in implementation, we introduce an error parameter $\epsilon$ in IP (Algorithm~\ref{algo:update}) to compare the floating numbers. %, i.e., we use $|a-b|\le \epsilon$ to replace $a=b$. 
Thus, we report the effect of error parameter $\epsilon$ on the result of estimated spread and time cost. 
We randomly select a vertex in \texttt{Facebook}, \texttt{DBLP} and \texttt{Youtube} as the seed to compute the influence spread and report the runtime, under TR model. 
Figure~\ref{fig:epsilona} shows the result of influence spread on different $\epsilon$, where the influence spread is almost the same (the difference is less than $0.1\%$) when $\epsilon < 10^{-9}$. 
%We also randomly select $100$ vertices as the seeds, and compute the average running time. 
Figure~\ref{fig:epsilonb} shows the runtime is related to the scale of the graph, and will gradually increase when $\epsilon$ increases. 
Therefore, we set $\epsilon=10^{-9}$ in all the experiments to trade-off the time cost and the accuracy. % performance of expected spread.

\begin{figure}[t]
    \centering
    \begin{subfigure}[h]{0.47\linewidth}
        \centering
        \includegraphics[width=1.0\textwidth]{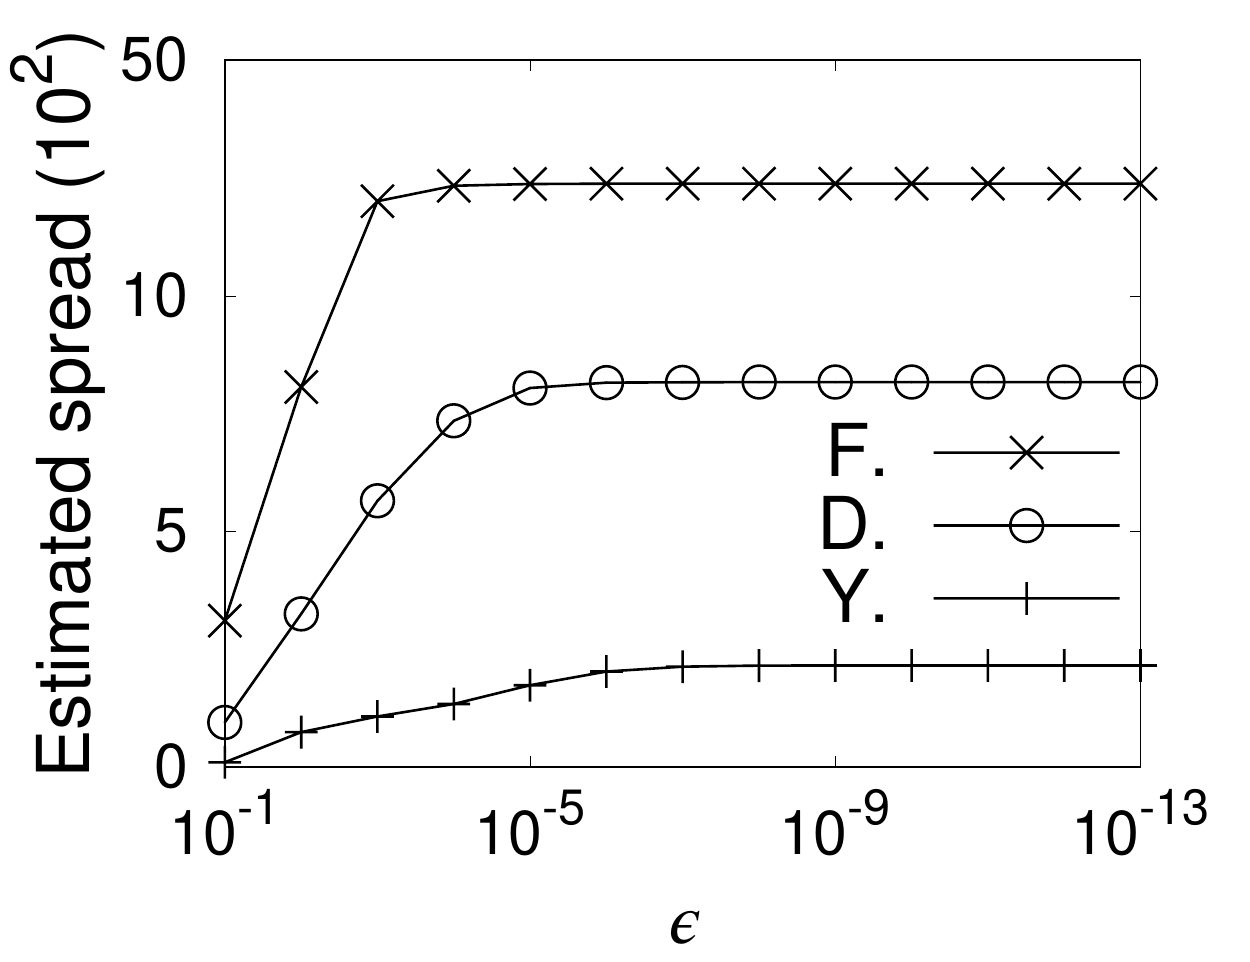}
        %\vspace{-1mm}
        \caption{Estimated spread}\label{fig:epsilona}
     %   \end{minipage}
    \end{subfigure}
    \begin{subfigure}[h]{0.47\linewidth}
        \centering
        \includegraphics[width=1.0\textwidth]{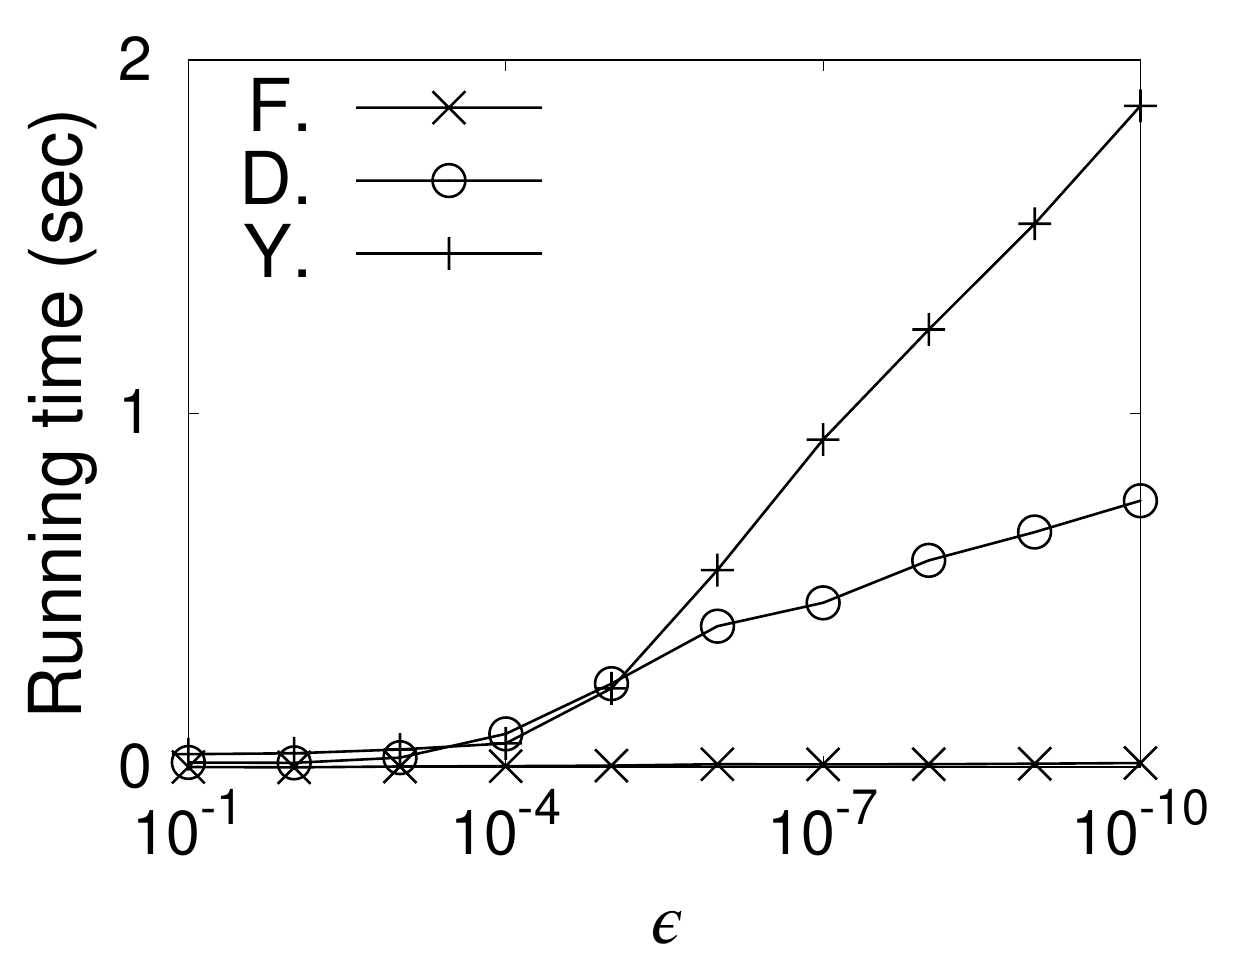}
        %\vspace{-1mm}
        \caption{Time cost}\label{fig:epsilonb}
    %    \end{minipage}
    \end{subfigure}
    \centering
    \vspace{-2mm}
    \caption{Estimated spread and running time on different $\epsilon$}\label{fig:epsilon}
\end{figure}

\vspace{1mm}
\noindent \textbf{Iterative Round of IP.}
We randomly select one vertex as the seed vertex, and compute the number of iterative rounds of IP (the iterative round is described in Section~\ref{sec:IP}) with $\epsilon=10^{-9}$.
The results are shown in Table~\ref{tab:round-ip}. The largest number of rounds is no more than $60$ which is much smaller than the round number of MCS, e.g., $r=10000$.

\begin{table}[t]
    \centering
    \small
    \caption{Number of iterative rounds $(i_{max})$ on all the datasets}\label{tab:round-ip}
    \vspace{-2mm}
    %\resizebox{\linewidth}{!}{
    \begin{tabular}{|c|cccccccc|}
    \toprule
         &  EC. & F. & W. & EA. & D. & T. & S. &Y.\\ \midrule
       TR model & 30 & 27 & 44 & 33 & 18 & 55 & 26 & 30   \\ \hline
       WC model & 12 & 25 & 20 & 40 & 25 & 60 & 29  & 31 \\
       \bottomrule
    \end{tabular}
    %}
\end{table}

\begin{figure}[t]
    \centering
    \begin{subfigure}[h]{0.47\linewidth}
        \centering
        \includegraphics[width=1.0\textwidth]{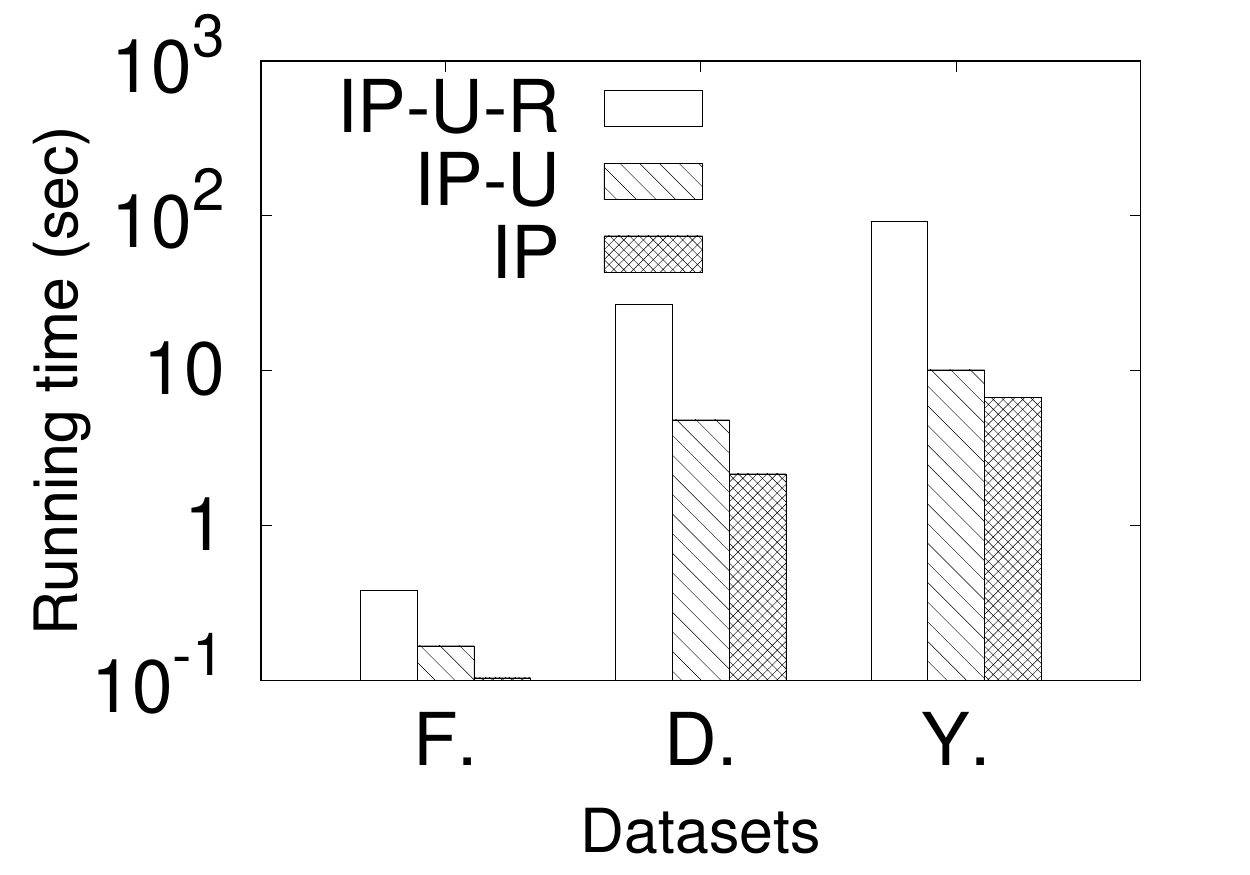}
        \caption{Time cost}\label{fig:estimea}
    \end{subfigure}
    \begin{subfigure}[h]{0.47\linewidth}
        \centering
        \includegraphics[width=1.0\textwidth]{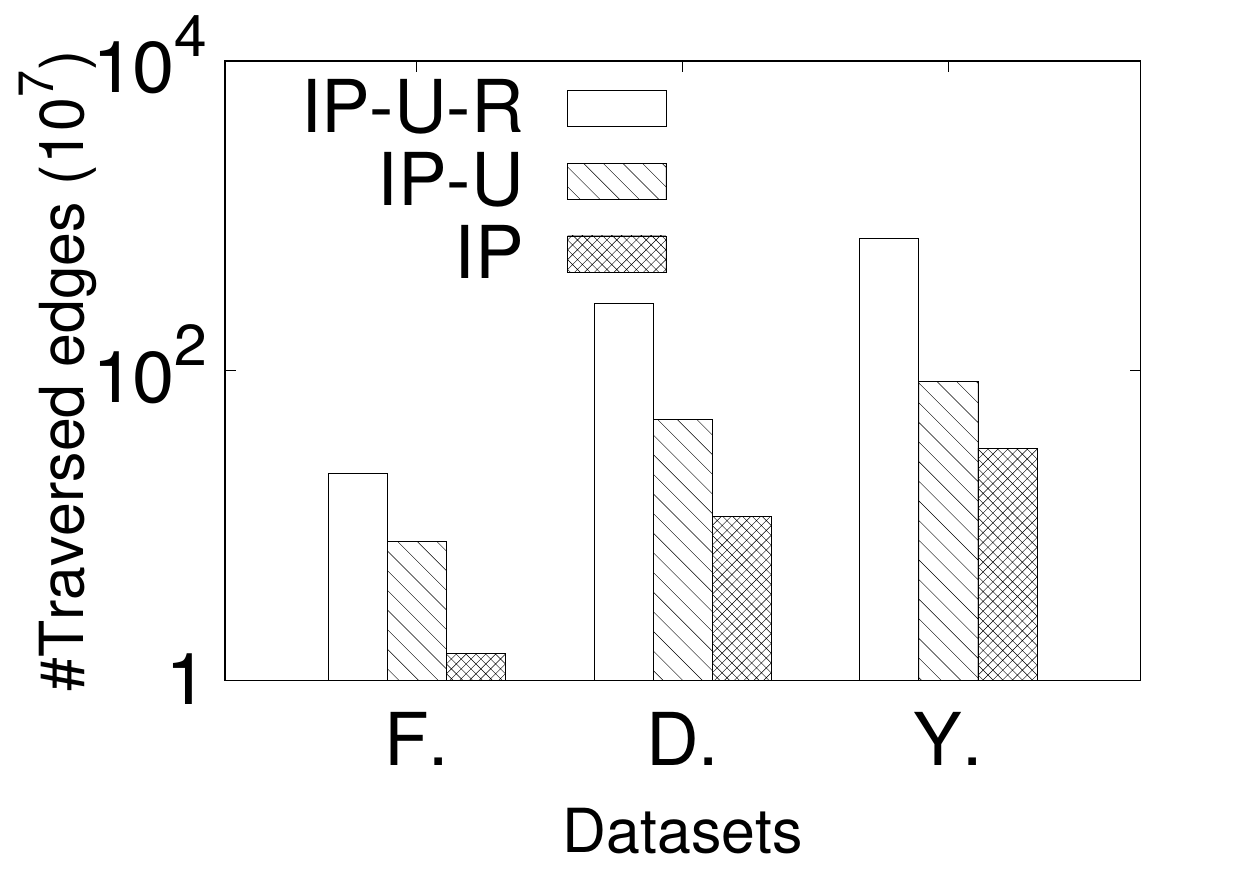}
        \caption{Traversed edges}\label{fig:estimeb}
    \end{subfigure}
    \centering
    \vspace{-2mm}
    \caption{Evaluating optimization techniques of IP}\label{fig:estime}
\end{figure}

\begin{table*}[t]
	\centering%
    %\vspace{-1mm}
	%\renewcommand{\arraystretch}{1.3}%
	\caption{Influence spread of different algorithms under WC model}\label{tab:im-wc}
%\begin{subtable}[h]{\linewidth}
\vspace{-3mm}
     \centering
	\resizebox{\linewidth}{!}{
	\begin{tabular}{|c|ccc|ccc|ccc|ccc|ccc|ccc|ccc|ccc|}
	\toprule
	&  \multicolumn{3}{|c|}{EC.}&  \multicolumn{3}{|c|}{F.}&  \multicolumn{3}{|c|}{W.}&  \multicolumn{3}{|c|}{EA.}&  \multicolumn{3}{|c|}{D.}&  \multicolumn{3}{|c|}{T.}&  \multicolumn{3}{|c|}{S.}&  \multicolumn{3}{|c|}{Y.} \\ \hline
$b$  &  GI  &  RL  &  MOVE  &  GI  &  RL  &  MOVE  &  GI  &  RL  &  MOVE  &  GI  &  RL  &  MOVE  &  GI  &  RL  &  MOVE  &  GI  &  RL  &  MOVE  &  GI  &  RL  &  MOVE  &  GI  &  RL  &  MOVE  \\ \midrule
20 & \bf{27.1} & 29.1 & \bf{27.1} & 197 & 196 &  \bf{194}  & \bf{20.1} & 21.2 & \bf{20.1} &  -  & 210 & \bf{207} &  -  & 272 & \bf{270} &  -  & 106 & \bf{104} &  -  & 344 & \bf{343} &  -  & 1372 & \bf{1334} \\ \hline
40 & 7.82 & 7.80 &  \bf{7.77}  & 141 & 141 &  \bf{138}  & \bf{14.3} & 16.1 & \bf{14.3} &  -  & 180 & \bf{166} &  -  & 104 & \bf{98.9} &  -  & 43.3 & \bf{41.0} &  -  & 190. & \bf{186} &  -  & 1205 & \bf{1161} \\ \hline
60 & 1.86 & 1.69 &   \bf{1.68}  & 110 & 109 &  \bf{108}  & 11.7  & 12.0 &  \bf{11.5}  &  -  & 97.2 & \bf{77.2} &  -  & 56.0 & \bf{21.6} &  -  & 31.6 & \bf{30.6} &  -  & 12.4 & \bf{11.7} &  -  & 1045 & \bf{922} \\ \hline
80 & 0.42 &  \bf{0.33} &  \bf{0.33} & 79.7 &  \bf{78.7}  &  \bf{78.7}  & 9.81 & 9.81 &  \bf{9.80}  &  -  & 90.0 & \bf{64.2} &  -  & 27.3 & \bf{15.1} &  -  & 5.40 & \bf{5.08} &  -  & 11.9 & \bf{9.37} &  -  & 1007 & \bf{709} \\ \hline
100 & 0 & 0 & 0 & 61.9 & \bf{61.1}  & \bf{61.1}  & 8.07 & 8.07 &  \bf{8.05}  &  -  & 37.7 & \bf{32.0} &  -  & 15.0 & \bf{7.65} &  -  & 0.68 & \bf{0.41} &  -  & 2.70 & \bf{2.04} &  -  & 981 & \bf{215} \\ \hline
	\bottomrule
	\end{tabular} }
  %  \caption{WC model}\label{tab:es-im-wc}
%\end{subtable}
\end{table*}

\vspace{1mm}
\noindent \textbf{Evaluating Optimization Techniques of IP.}
We compare the following algorithms by randomly remove a vertex and restore a vertex that has been removed under TR model, for $100$ independent tests: (i) \textbf{IP}: our final IP algorithm (Algorithm~\ref{algo:IP}); (ii) \textbf{IP-U}: \texttt{IP} without applying Algorithm~\ref{algo:update}, i.e., the computation of activation probabilities starts from $ap[s]=1$ and $ap[u]=0$ for each $u\neq s$; (iii) \textbf{IP-U-R}: \texttt{IP} without pruning the invalid updates (Section~\ref{sec:IP}). 

Figure~\ref{fig:estimea} shows the running time of the algorithms on three datasets.
Figure~\ref{fig:estimeb} reports the number of traversed edges for updating the activation probabilities. 
The results show \texttt{IP-U} is faster than \texttt{IP-U-R} by around $1$ order, with equipping the pruning technique. 
Benefiting from reusing the intermediate results, \texttt{IP} is faster than \texttt{IP-U} by more than $2$ times. 
The speedup is also validated by the difference on the number of traversed edges.
%And the number of traversed edges mean the amount of calculation of expected spread, showing the same law. 
%Besides, the gap between \texttt{IP} and \texttt{IP-U-R} will even become larger as the scale of dataset increases.

\begin{figure}[t]
    \centering
    \begin{subfigure}[h]{0.47\linewidth}
        \centering
        \includegraphics[width=1.0\textwidth]{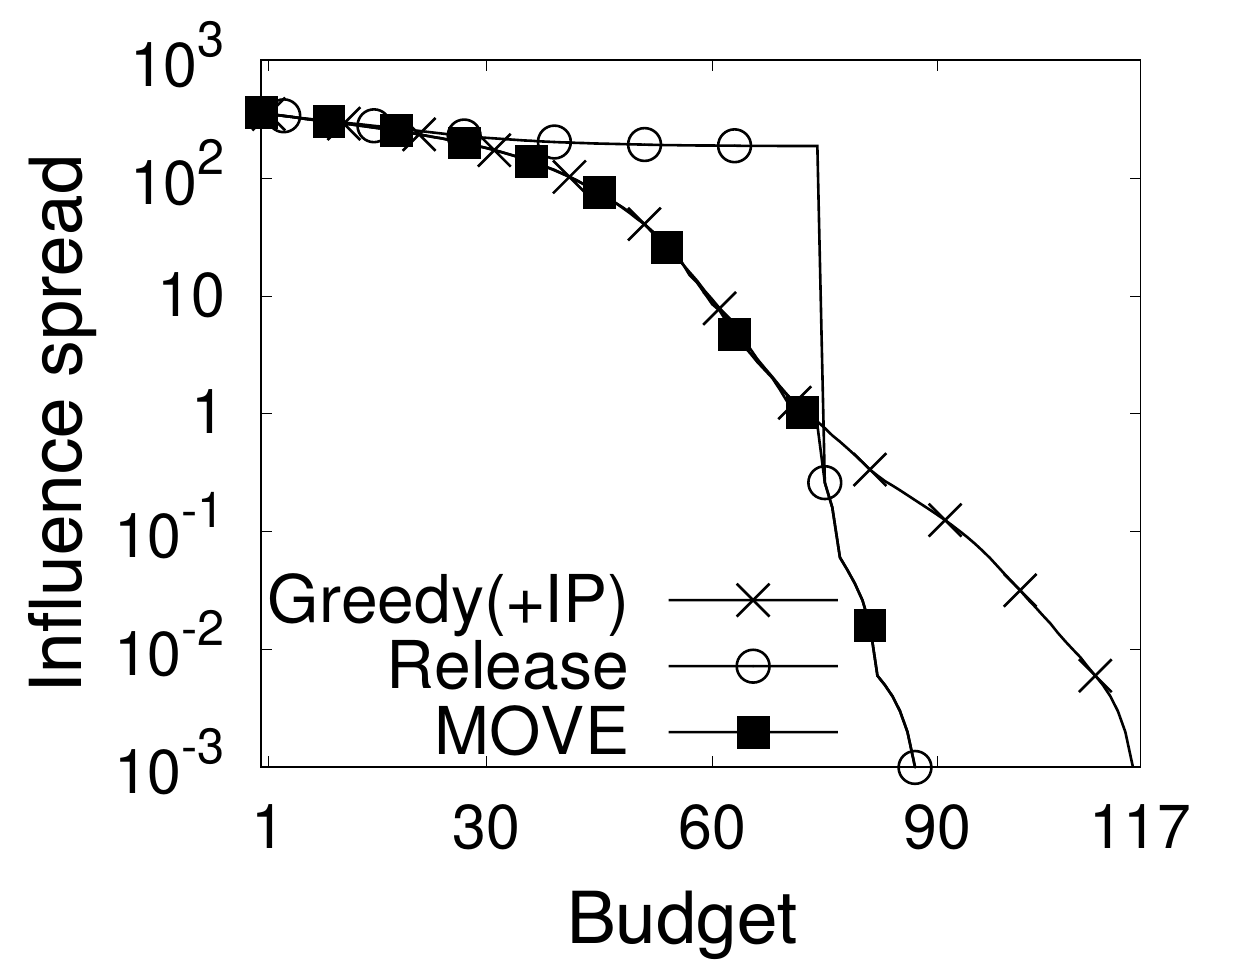}
        \caption{\texttt{EmailCore}: Influence spread}\label{fig:im-tra}
    \end{subfigure}
    \begin{subfigure}[h]{0.47\linewidth}
        \centering
        \includegraphics[width=1.0\textwidth]{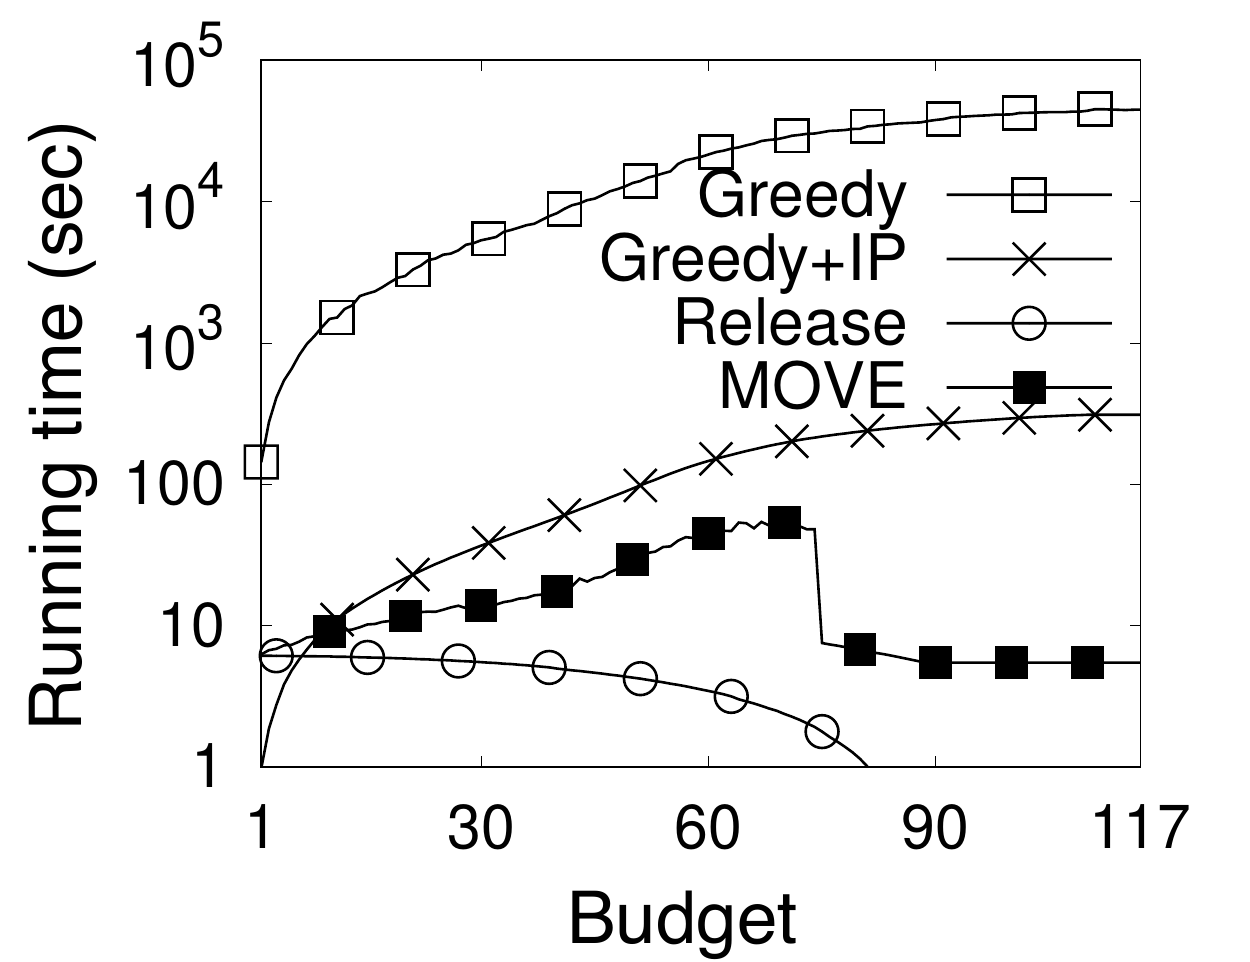}
        \caption{\texttt{EmailCore}: Time cost}\label{fig:im-trb}
    \end{subfigure}
    \begin{subfigure}[h]{0.47\linewidth}
        \centering
        \includegraphics[width=1.0\textwidth]{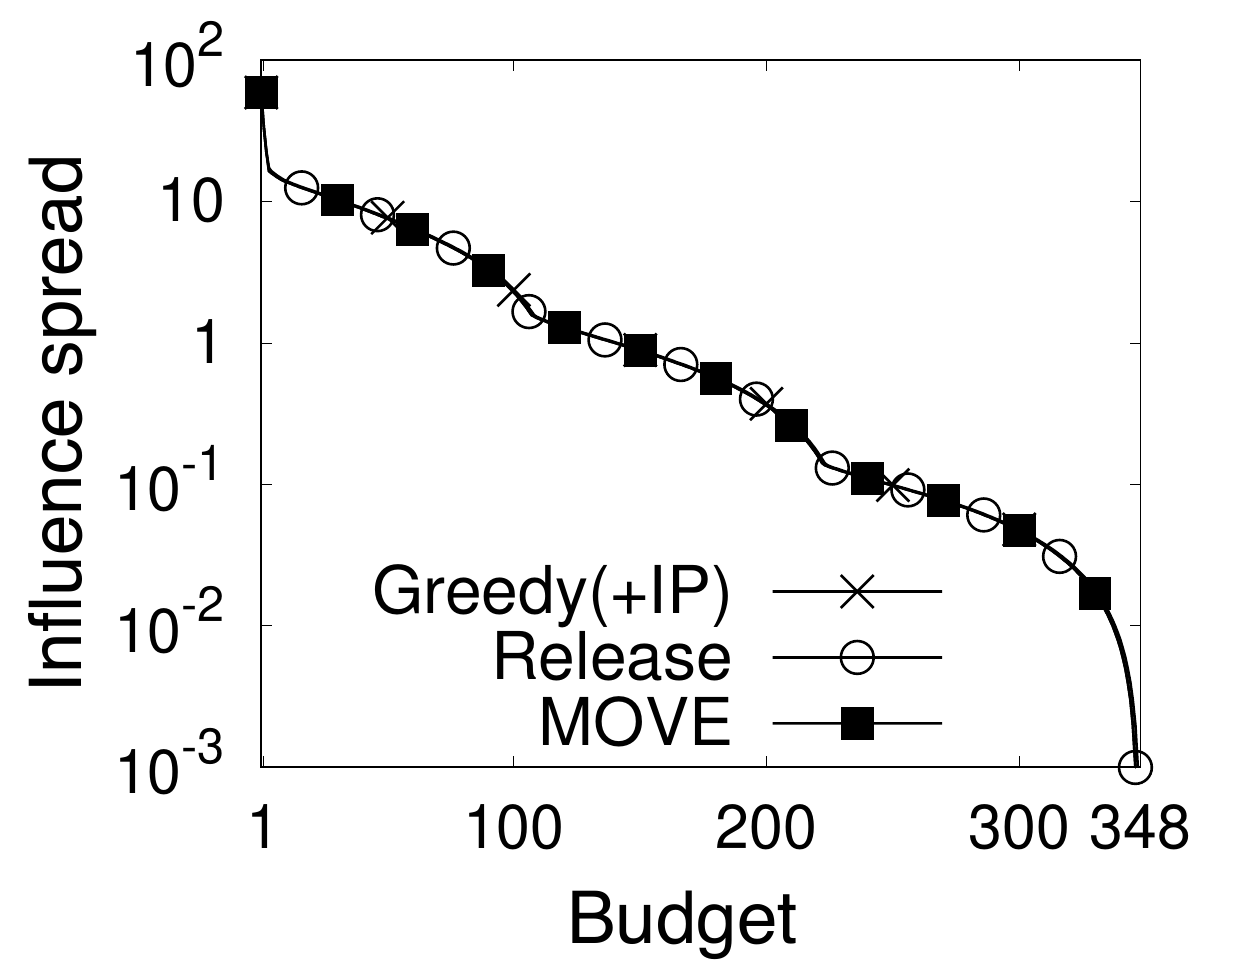}
        \caption{\texttt{Facebook}: Influence spread}\label{fig:im-trc}
    \end{subfigure}
    \begin{subfigure}[h]{0.47\linewidth}
        \centering
        \includegraphics[width=1.0\textwidth]{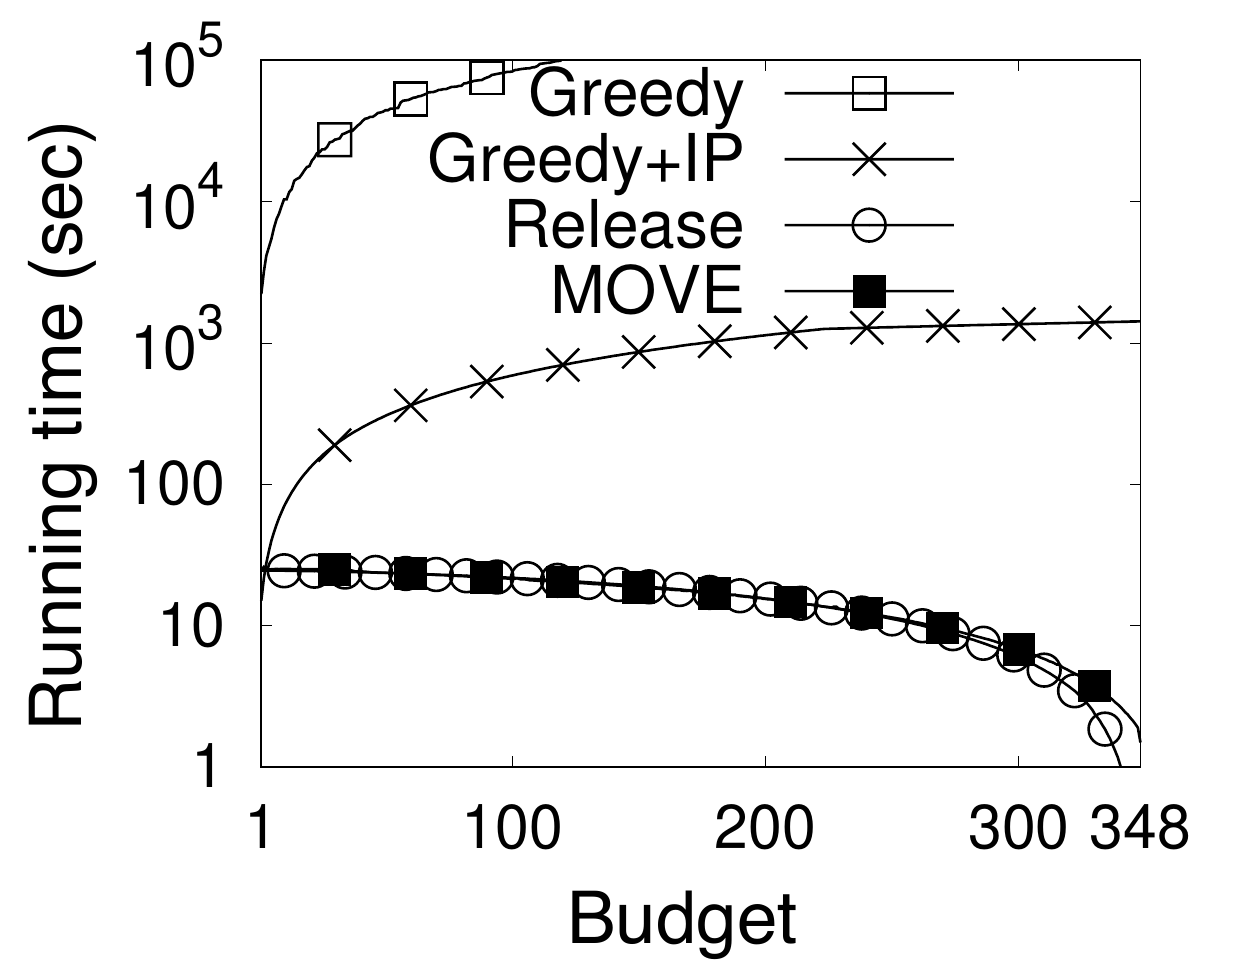}
        \caption{\texttt{Facebook}: Time cost}\label{fig:im-trd}
    \end{subfigure}
    \centering
    \caption{Influence spread and time cost under different $b$}\label{fig:im-tr}
\end{figure}

\vspace{1mm}
\noindent \textbf{Varying Budget $b$.}
Figure~\ref{fig:im-tr} shows the resutls of influence spread and time cost for four algorithms under TR model, by varying the budget $b$.
As Greedy can only handle small graphs, we report the results on {EmailCore} and {Facebook}.
Figure~\ref{fig:im-tra} shows Greedy performs well on small $b$, Release outperforms Greedy on large $b$, and MOVE algorithm well combines the advantages of Greedy and Release. Note that the spread is almost same for Greedy and Greedy+IP.
Figure~\ref{fig:im-trb} shows IP can largely speeds up Greedy and MOVE achieves a good trade-off between result quality and time cost.
The running time of the MOVE algorithm drops at $b=75$, because its initial blockers are close to the optimal results and the cost of move operation becomes small.
In Figure~\ref{fig:im-trc}, the spreads are similar for all the algorithms because they all find near-optimal results.
In Figure~\ref{fig:im-trd}, the runtime of MOVE is close to Release, which is much smaller than the greedy algorithms.

% while the MOVE algorithm does not need much time to MOVE the blockers. 
% We only show part of running time of Greedy in Figure~\ref{fig:im-trd} because of its large computation cost. 
% Although our IP algorithm helps the Greedy+IP fast than Greedy $2-3$ orders, the MOVE still costs less time than the Greedy+IP algorithm when the budget is large, and shows the opposite trend with increasing budgets. 
% Figure~\ref{fig:im-tra} and Figure~\ref{fig:im-trb} show both expected spread and running time of the MOVE algorithm seriously drop at \#Budgets$=75$, because the blockers are becoming close to the seed vertex while the MOVE algorithm does not need much time to MOVE the blockers. 
% Figure~\ref{fig:im-tra} also shows MOVE algorithm needs fewer budgets to dispel the influence of rumors.

\begin{figure}[t]
    \centering
    \begin{subfigure}[t]{0.47\linewidth}
        \centering
        \includegraphics[width=1.0\textwidth]{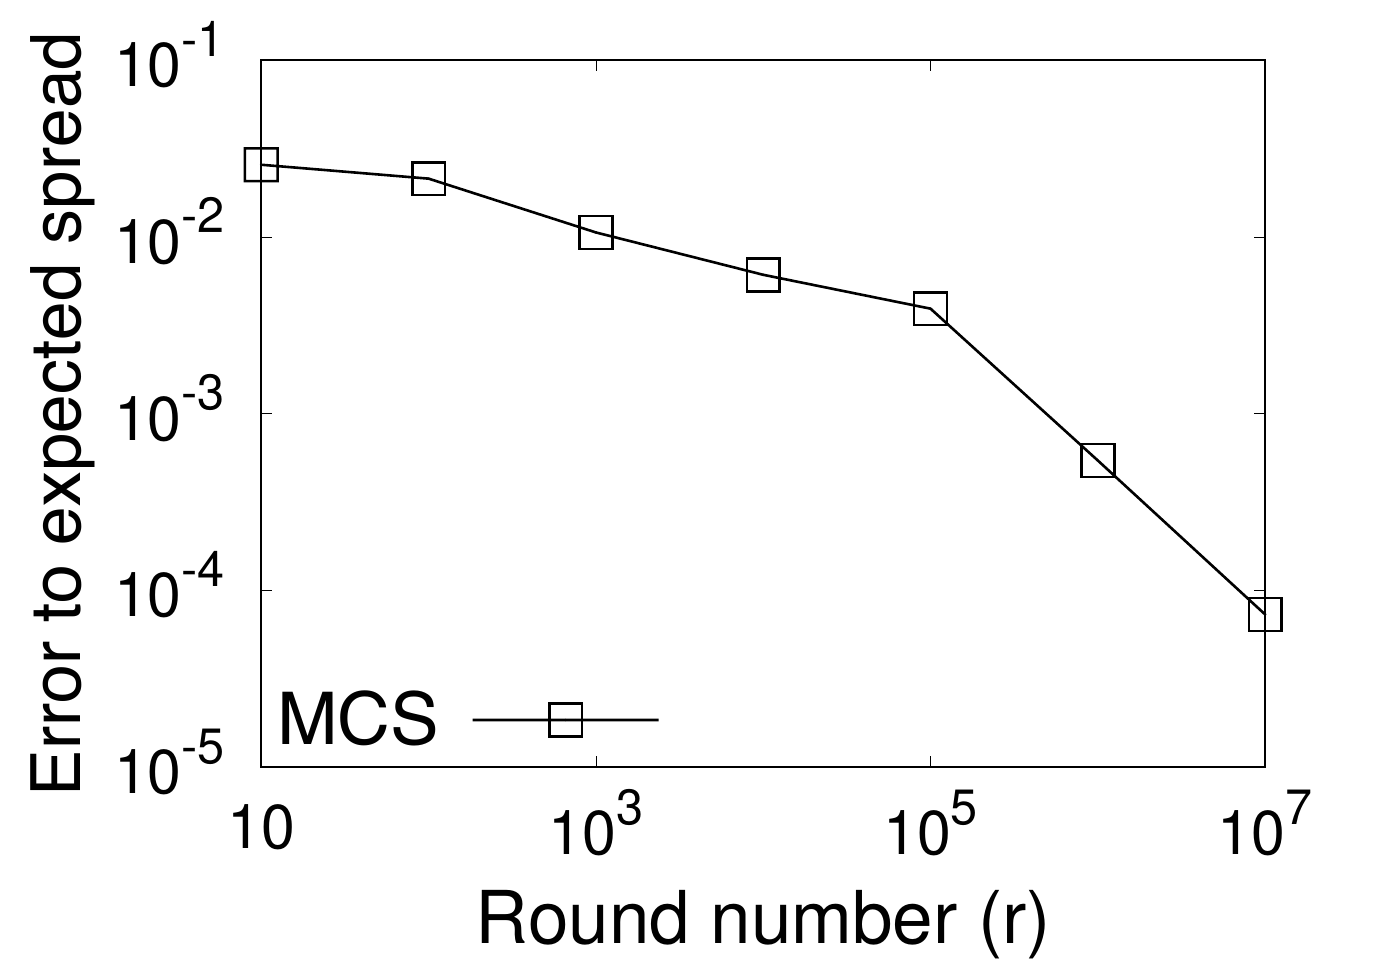}
        \caption{Monte-Carlo Simulations}\label{fig:IP-exacta}
    \end{subfigure}
    \begin{subfigure}[t]{0.47\linewidth}
        \centering
        \includegraphics[width=1.0\textwidth]{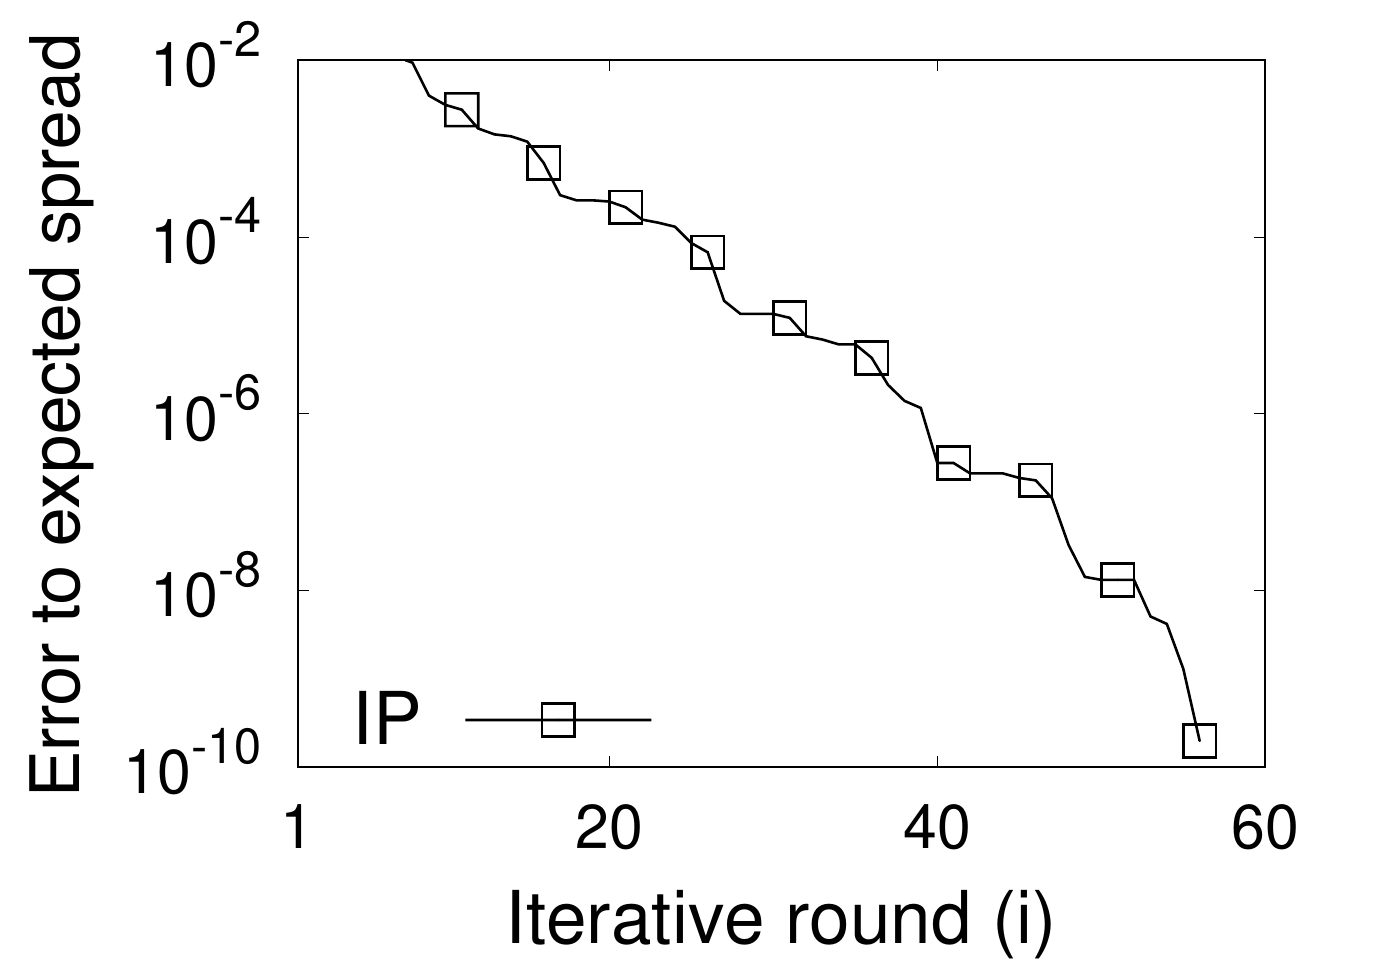}
        \caption{Iterative Progress}\label{fig:IP-exactb}
    \end{subfigure}
    \centering
    \vspace{-3mm}
    \caption{Accuracy (WC model): MCS v.s. IP}\label{fig:IP-exact-wc}
\end{figure}

%\subsection{Additional Results under }
%For all the experiments in Section~\ref{sec:exp}, the corresponding results under WC model are as follows.

\vspace{1mm}
\noindent \textbf{Accuracy of Iterative Progress (WC Model).}
We extract small datasets from \texttt{EmailCore} where each dataset is an induced subgraph of 50 random vertices. Figure~\ref{fig:IP-exact-wc} (referred in Section~\ref{sec:epsilon}) shows the error of estimated spread by Iterative Progress and Monte-Carlo Simulations, where $10$ random vertices are set as the seeds. 
For an error in the order of $i = 10^{-3}$, the round number of IP is about 10 while the round number can be $r = 10^6$ for MCS. %, and IP is much faster than MCS.

\vspace{1mm}
\noindent \textbf{Efficiency of Iterative Progress (WC Model).}
We set $r=10000$ for MCS and $\epsilon = 10^{-9}$ for IP. 
Figure~\ref{fig:mc-wc} (referred in Section~\ref{sec:epsilon}) shows the average running time of a random vertex under WC model, where IP is faster than MCS by $2$-$3$ orders of magnitude.

\begin{figure}[t]
    \centering
%\subfigure[Expected Spread]{
        \begin{minipage}[h]{0.9\linewidth}
        \centering
        \includegraphics[width=1.0\textwidth]{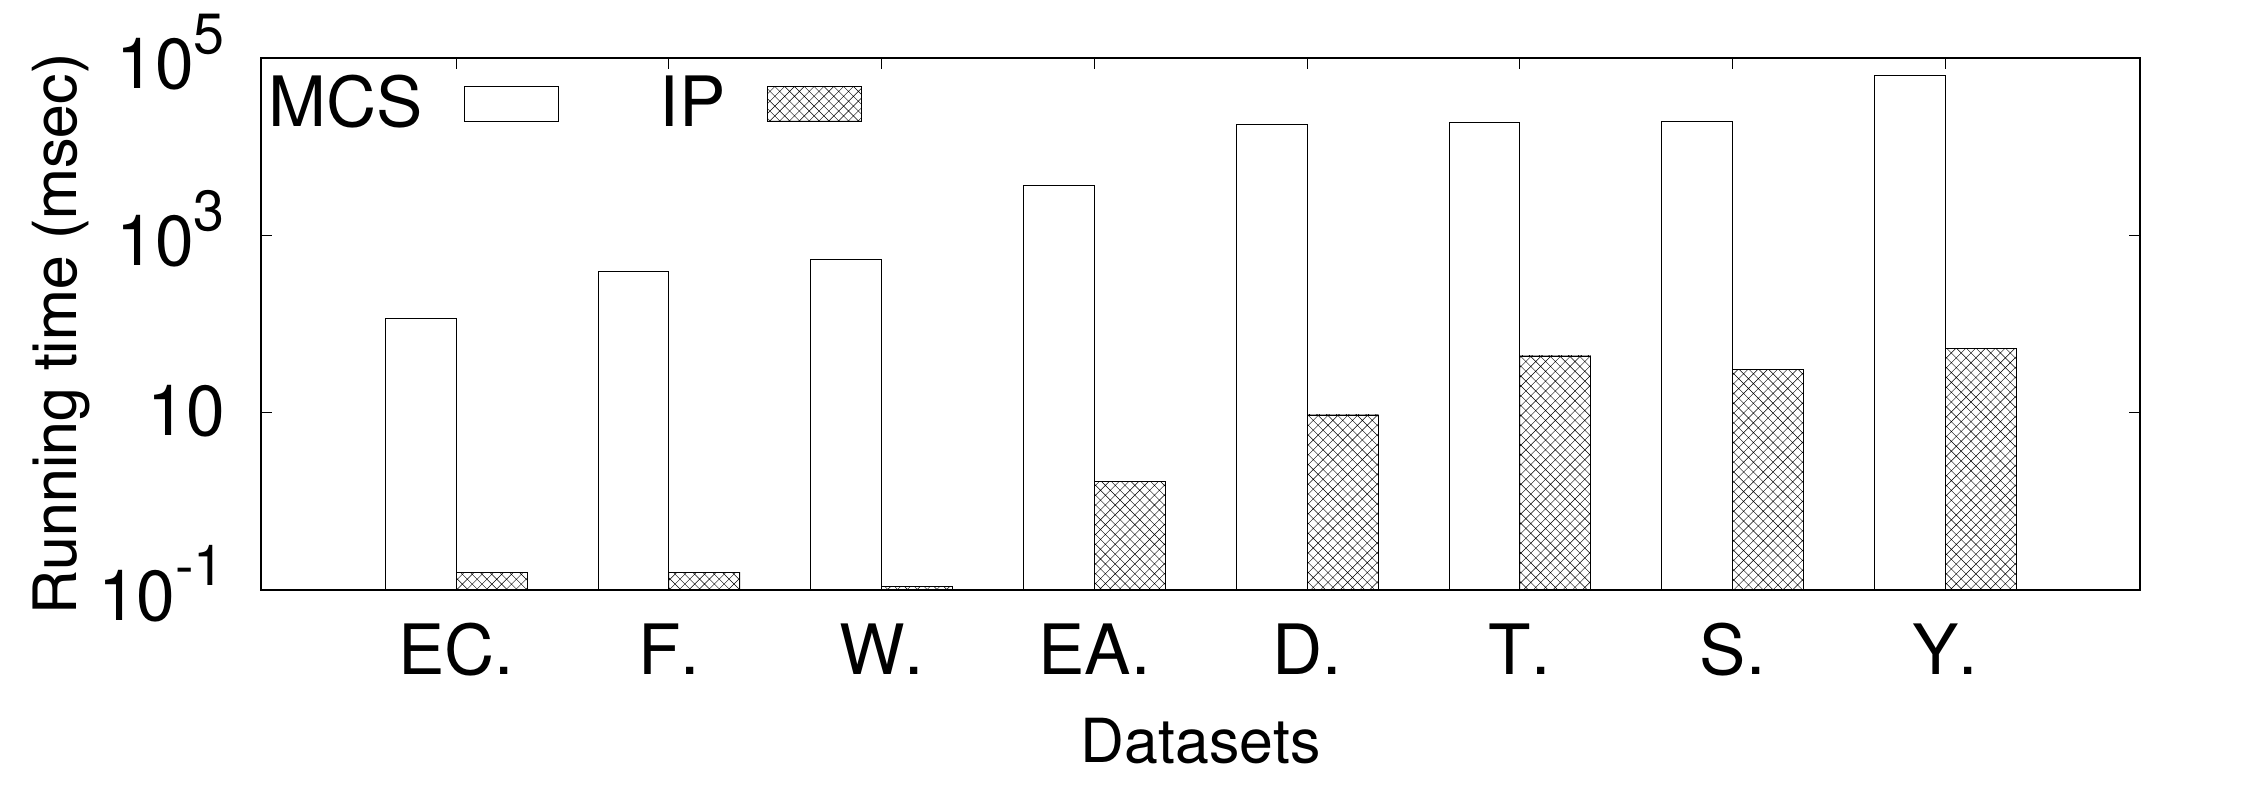}
        \end{minipage}
    %}
    \centering
    \vspace{-3mm}
    \caption{Average runtime (WC model): MCS v.s. IP}\label{fig:mc-wc}
\end{figure}

\vspace{1mm}
\noindent \textbf{Influence Spread of MOVE (WC Model).}
We randomly select $10$ vertices as the seeds.
Table~\ref{tab:im-wc} (referred in Section~\ref{sec:exp-im}) shows the average influence spread of three different algorithms. MOVE always returns the best result due to its lowest influence spread. Although Release algorithm performs well in three small datasets (similar to the performance of MOVE), the gap becomes larger between Release and MOVE on larger datasets.

\vspace{1mm}
\noindent \textbf{Time Cost of MOVE (WC Model).}
Figure~\ref{fig:im-time-wc} (referred in Section~\ref{sec:exp-im}) shows the average running time of 4 algorithm on each dataset, when the budget $b$ is $100$. 
The performance of each algorithm is similar to the result under TR model.

\begin{figure}[t]
    %\begin{subfigure}[h]{0.47\linewidth}
        \centering
        \begin{minipage}[h]{0.9\linewidth}
        \centering
        \includegraphics[width=1.0\textwidth]{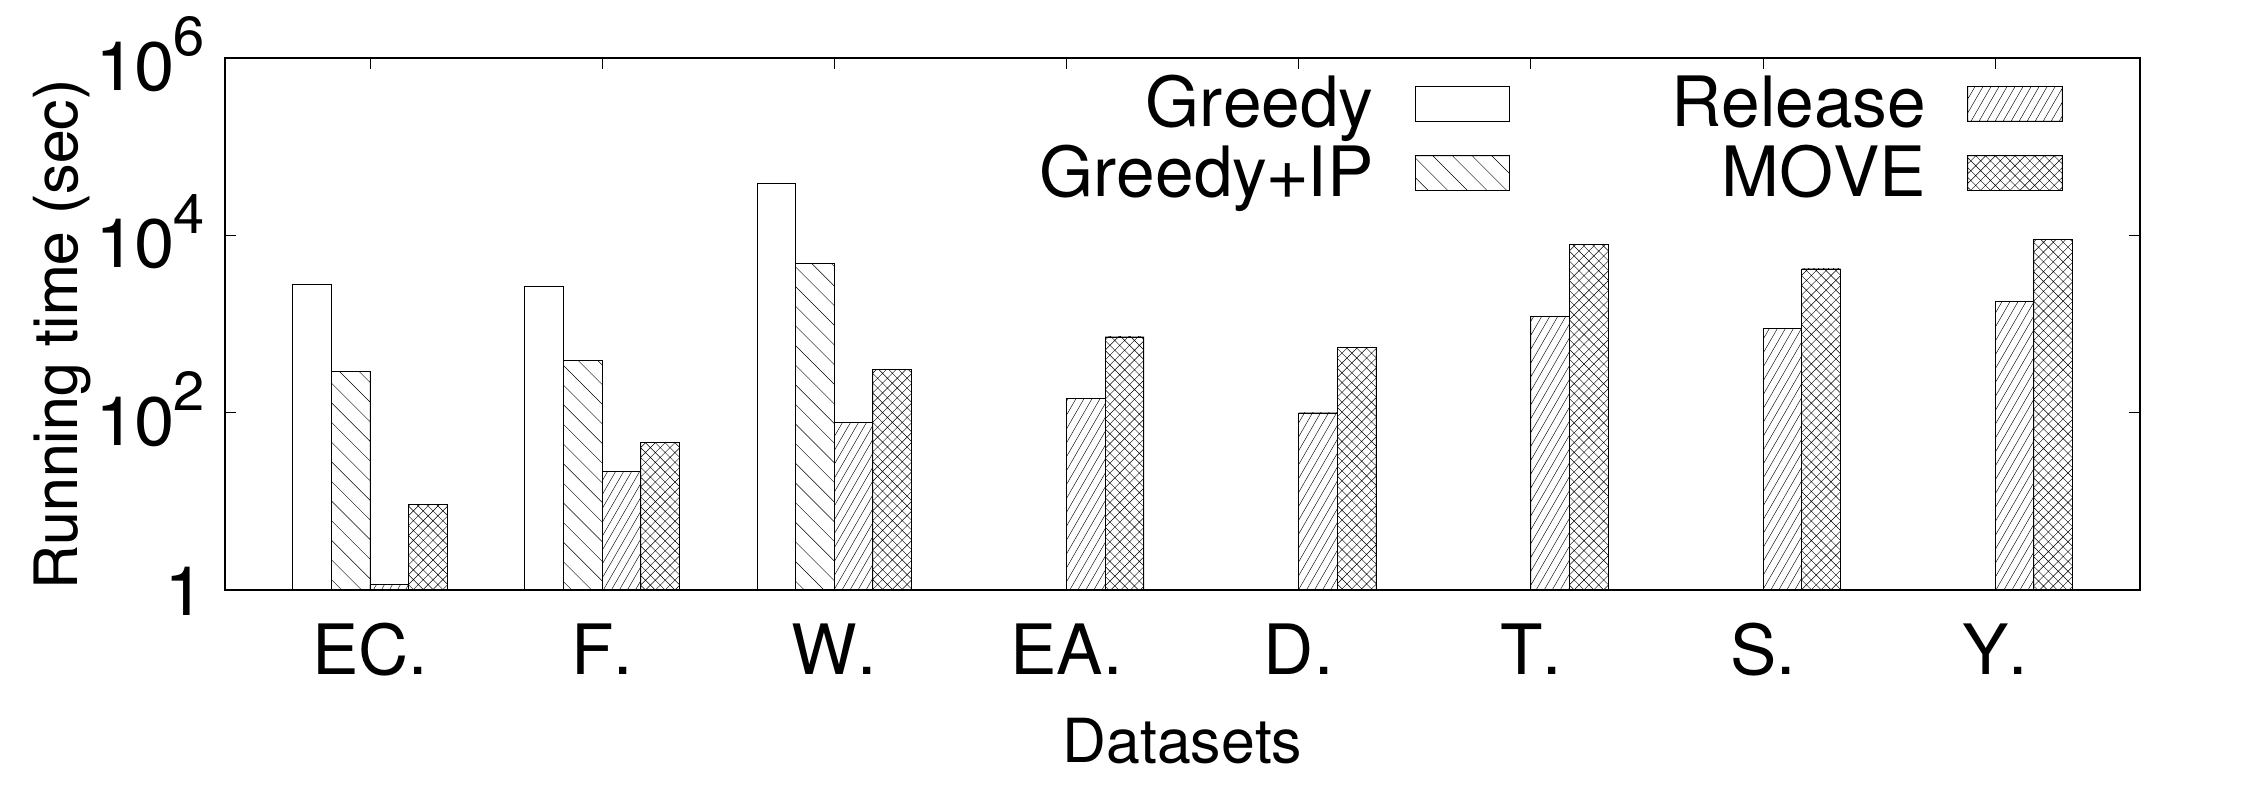}
        \end{minipage}
        \vspace{-3mm}
        \caption{Average runtime, $b=100$ (WC model)}\label{fig:im-time-wc}
    %\end{subfigure}
    %\caption{Average Time cost of different algorithms}\label{fig:im-time}
\end{figure}
